# Supplementary material for: FlowDubber: Movie Dubbing with LLM-based Semantic-aware Learning and Flow Matching based Voice Enhancing
Source: arXiv:2505.01263 source file (2025-08-25)
Supplement: Supplementary file 1 [file x_appendix.tex]

\appendix

\section{Theoretic Details of Flow Matching}\label{flowmatching}

Given the mel-spectrograms data space with data point $M$, where $M \sim q(M)$ and $q(M)$ is an unknown data distribution of mel-spectrograms, a possible approach to sample $M$ from $q(M)$ is from the probability density path defined as $p_t(x)$ where $t\in [0,1]$, $p_0(x)=\mathcal{N}(x;\boldsymbol{0},\boldsymbol{I})$ and $p_1(x)\approx q(x)$.
To estimate the probability density path, Continuous Normalizing Flow~\cite{chen2018neural} defines a vector field $v_t$, which gives a flow $\phi_t(x)$ through an Ordinary Differential Equation (ODE):
%Conditional Flow Matching (CNF)~\cite{lipman2022flow} defines a vector field $v_t$, which gives a flow $\phi_t(x)$ through an Ordinary Differential Equation (ODE):
%Given $\mu \in\mathbb{R}^{{M_l}\times{d_a}}$ in Eq. ~\ref{eq:mu_cond} as the condition and mel-spectrogram $M$ as the corresponding data, Conditional Flow Matching (CNF)~\cite{lipman2022flow} defines a vector field $v_t$, which gives a flow $\phi$ that satisfies:
\begin{equation}
    \frac{d}{dt}\phi_t(x)= v_t(\phi_t(x)); \quad \phi_0(x)=x. 
\end{equation}
%where the initial condition is $\phi_0(x)=x$. 
\citet{chen2018neural} shows that predicting the vector flow $v_t$ through a neural network $\theta$ can be used to transform a simple Gaussian distribution to a more complicated one, such as $q(x)$, which generates the probability density path. Flow matching is designed to predict such a probability density path. Give a target probability density path $p_t$ with its corresponding known vector field $u_t(x)$, 
the training objective of flow matching is:
\begin{equation}
    \mathcal{L}_{FM}(\theta)=\mathbb{E}_{t,p_t(x)}||v_t(x,\theta)-u_t(x)||^2
\end{equation}

However, the total probability density path $p_t$ is unknown and we can only use some samples from $q(x)$ to estimate the probability density path, which is Conditional Flow Matching (CFM). The training objective of CFM is:
\begin{equation}
    \mathcal{L}_{CFM}(\theta)=\mathbb{E}_{t,M\sim q(M),p_t(x|M)}||v_t(x,\theta)-u_t(x|M)||^2,
\end{equation}

We can efficiently estimate the probability density path $p_t(x)$ by sampling from $q(M),p_t(x|M)$ and calculate $u_t(x|M)$. Here we use optimal-transport conditional flow matching (OT-CFM) to train our model, which is a simple version of CFM with simple flow $\phi_t(x)=(1-(1-\sigma_{\min})t)x_0+tM$, which satisfies $x_0\sim \mathcal{N}(x;\boldsymbol{0},\boldsymbol{I})$ and $\phi_1(x)\sim q(x)$. Its gradient vector field is $u_t(\phi_t(x)|M)=M-(1-\sigma_{min})x_0$, enabling fast training and inference for its linear and time-invariant properties. Given conditional mean $\mu$, the training objective of OT-CFM can be formulated as:
\begin{equation}
\mathcal{L_\theta}=\mathbb{E}_{t,q(M),p_t(x|\mu,M)} ||v_t(\phi_t(x)|\mu,\theta)-u_t(\phi_t(x)|M)||^2,
\end{equation}
where $v_t(\phi_t(x)|\mu,\theta)$ is the predicted gradient vector field of $\phi_t(x)$ according to the acoustics prior information $\mu$. Then, we can solve the ODE $d\phi_t(x)=v_t(\phi_t(x)|\mu,\theta)dt$ from $t=0$ to $t=1$ to generate the target mel-spectrogram $\hat{M}$ from noise $x_0$. 

\begin{table}[!t]
  \centering
    \caption{Subjective evaluation on GRID benchmark.}
    \vspace{-0.2cm}
  {
    \begin{tabular}{c|ccc}
    \hline
    Dataset & \multicolumn{3}{c}{GRID} \\ 
    \toprule
    Methods 
    & MOS-N $\uparrow$
    & MOS-S $\uparrow$ 
    & CMOS $\uparrow$  \\
  
    \midrule
    GT   &  4.69$\pm$0.07 & - & +0.10 \\
    \midrule
    V2C-Net~\cite{chen2022v2c}  & 3.62$\pm$0.06 & 3.67$\pm$0.11 &-0.35 \\
    HPMDubbing~\cite{cong2023learning} & 3.77$\pm$0.20 & 3.74$\pm$0.13 &-0.26 \\
    StyleDubber~\cite{cong2024styledubber} & 4.02$\pm$0.11 & 4.06$\pm$0.05 &-0.19\\
    \midrule
    Speaker2Dubber~\cite{zhang2024speaker}  & 4.10$\pm$0.09 & 4.05$\pm$0.11 &-0.18 \\
    Produbber~\cite{zhang2025produbber} & 4.12$\pm$0.07  & 4.07$\pm$0.10 & -0.13\\
    \midrule
     Our method &   \textbf{4.15$\pm$0.06}  &  \textbf{4.10$\pm$0.07}  &  \textbf{0.00}  \\
    \bottomrule
    \end{tabular}
    }
  \label{result_MOS}
  \vspace{-0.8mm}
\end{table}% 

\section{LSE or MCD-DTW-SL for measuring lip-sync?}
% \label{discusss_SL_L}

MCD-DTW-SL cannot truly measure audiovisual synchronization because the coefficients of MCD-DTW-SL are based on the global time rather than the fact to reflect the alignment related to lip movement. 
Below is the formula of MCD-DTW-SL: 
\begin{equation}\label{eq:adv_MCD_DTW}
    %\begin{aligned}
        \text{MCD-DTW-SL} (\mathcal{C}, \mathcal{C}') =  \frac{\eta}{R} \cdot \gamma_{M,N}.
     %\end{aligned}
     % \vspace{-5pt}
\end{equation} 
where the $\mathcal{C}= \{\mathbf{c}_1, \mathbf{c}_2, ..., \mathbf{c}_i, ..., \mathbf{c}_M\}$ and $\mathcal{C}'=\{\mathbf{c}'_1, \mathbf{c}'_2, ..., \mathbf{c}'_j, ..., \mathbf{c}'_N\}$ represent the generated speech and ground truth of Mel Frequency Cepstral Coefficient (MFCC) vectors, respectively. 
The $M$ and $N$ denote the length of MFCC vectors of generated speech and ground truth, respectively. 
The $\gamma_{M,N}$ represents the objective minimum distance by accumulating $R$ distances in total between $\mathcal{C}$ and $\mathcal{C}'$ via Dynamic Time Warping (DTW)~\cite{muller2007dynamic} algorithm. 
In other words, the $\text{MCD-DTW-SL} (\mathcal{C}, \mathcal{C}') =  \eta \cdot \text{MCD-DTW} (\mathcal{C}, \mathcal{C}')$, where the $\eta=\frac{\text{max}(M,N)}{\text{min}(M,N)}$ indicates the coefficient ratio of the total length of the two audio segments $\mathcal{C}$ and $\mathcal{C}'$. 
That means if the two audio clips are exactly equal, then $\text{MCD-DTW} (\mathcal{C}, \mathcal{C}')$ is equal to $\text{MCD-DTW-SL} (\mathcal{C}, \mathcal{C}')$. 
For dubbing tasks, since the total dubbing times (the length of mel-spectrograms $T_{mel}$) can known by multiplying time coefficient $n$ with video frames $T_v$ in advance~\cite{hu2021neural}:
\begin{equation}
    \begin{aligned}
        n = \frac{T_{mel}}{T_v}=\frac{sr/hs}{FPS} \in \mathbb{N}^{+},
     \end{aligned}
\end{equation}
where $FPS$ denotes the Frames per Second of the video, $sr$ denotes the sampling rate of the audio, and $hs$ denotes hop size when transforming the raw waveform into mel-spectrograms. 
In this case, the audio length is known in advance, MCD-DTW-SL is meaningless for determining alignment. 
Thus, we encourage evaluating the audio-visual synchronization in movie dubbing by using metrics LSE-D and LSE-C, which are widely adopted for quantitative evaluation of lip-syncing performance in the wild~\cite{DogucanAudioVisual, TaekyungStyleLipSync, XiaodaSyncTalklip, JintaoLandmark, ParkExploring}. 
The LSE-D measures the distance between the audio and visual representations with lower scores suggesting better audio-visual sync. 
LSE-C is the confidence score, and the higher value implies a stronger correlation between video and speech~\cite{SongjuDubbing, YanLiuM3TTS, DubWiseNehaSahipjohn}.

\section{Subjective Evaluation on GRID
Benchmark}\label{discusss_SL_L} 

Since we only provide objective evaluation in the main paper,  we provide the subjective evaluation by human, following previous dubbing works~\cite{zhang2024speaker,zhang2025produbber}. 
Please note that the UTMOS and DNSMOS in the paper are given by the model prediction to ensure fairness, rather than human subjective evaluation. 

\noindent \textbf{MOS-N \& MOS-S.}
MOS-Naturalness (MOS-N) and MOS-Similarity (MOS-S) are mean option scores reported with a 95\% confidence interval based on ratings from 20 native English speakers using a scale from 1 to 5. 
Each participant is required to listen to 30 randomly selected generated dubbing and rate the dubbing according to the speech naturalness and voice similarity following~\cite{chen2022v2c}.

\noindent \textbf{CMOS.}
Comparative mean option score (CMOS) asks participants to compare the dubbing generated by two models using same input and rate them on a scale from -5 to 5 based on criterion of matched degree between generated dubbing with video~\cite{zhang2025produbber}.

Under the same experimental setting, we found that the proposed FlowDubber is also subjectively superior to the previous methods, especially in speech quality (MOS-N), indicating the best overall dubbing quality.
